# Supplementary material for: Collaborative Large and Small Language Models for Accurate and Scalable Data Repair
Source: arXiv:2606.17582 source file (2026-06-16)
Supplement: Supplementary file 1 [file 8_appendix.tex]

\section{Appendix}

\subsection{Effectiveness of the EM algorithm}
\label{subsec:em-effectiveness}

In Section~\ref{subsec:em}, we started Theorem~\ref{thm:em-monotone}, claiming that the EM refinement procedure is monotonic in the marginal log-likelihood. 

We only need to consider the log-likelihood of the observed data at iteration $t$. Let $\{(\theta^{(t)},\hat{\mathbf z}^{(t)})\}_{t\ge 0}$ be the sequence generated by the EM updates in Section~\ref{subsec:em}, where $\hat{\mathbf z}^{(t)}:=\{\hat z_{ij}^{(t)}\}_{(i,j)\in E}$. The log-likelihood of observed data is:
$$
\ell (\theta^{(t)}, z^{(t)}) = \log p_\theta(\mathbf{D})=\sum_{(i,j)\in\mathcal{E}} \log p_\theta(z_{ij}^{(t)} \;\big| \;x_i^{j}).
$$
% Tried to add a lemma here, but it does not make sense at all
% \begin{lemma}[EM lower bound]
% \label{lem: em_lb}
% For any collection of distributions $q={\{q\}_{(i,j)\in\mathcal{E}}}$ where $q_{ij}$
% \end{lemma}
Now we can restate the theorem and give the proof

\begin{theorem}[Restatement of monotonicity of EM]
Given the condition that both the Expectation and the maximization are ideal. We have the log-likelihood $\ell(\theta^{(t)}, z^{(t)})$ is monotonically non-decreasing along the iterations:
$$
\ell(\theta^{(t+1)},\hat{\mathbf z}^{(t+1)}) \ge \ell(\theta^{(t)},\hat{\mathbf z}^{(t)}),\qquad \forall t\ge 0.
$$
\end{theorem}

\begin{proof}
We consider one Expectation step and one maximization step.
\paragraph{Expectation improves $\ell$ for fixed $\theta^{(t)}$.} At iteration $t$, given current parameter $\theta^{(t)}$, for each $(i,j)\in \mathcal{E}$. $\hat z_{ij}^{(t)}=\arg\max_z p_{\theta^{(t)}}(z\mid x_i^{(j)})$ maximizes the log-likelihood. Hence,
\begin{align*}
    \ell(\theta^{(t)},\hat{\mathbf z}^{(t+1)}) &=\max_z p_{\theta^{(t)}}(z\mid x_i^{(j)})\\
    &\ge p_{\theta^{(t)}}(\hat{\mathbf z}^{(t)}\mid x_i^{(j)}) \\
    &=\ell(\theta^{(t)},\hat{\mathbf z}^{(t)}).
\end{align*}

\paragraph{maximization improves $\ell$ for fixed $\hat{\mathbf z}^{(t)}$.} By the definition of the maximization, 
\begin{align*}
    \theta^{(t+1)} &= \arg\max_{\theta}\sum_{(i,j)\in \mathcal{E}} \log p_{\theta}(\hat z^{(t)}_{ij}\mid x_i^{(j)}).
\end{align*}
Thus,
\begin{align*}
    \ell(\theta^{(t+1)},\hat{\mathbf z}^{(t+1)}) &=\max_\theta p_{\theta}(\hat{\mathbf z}^{(t+1)}\mid x_i^{(j)})\\
    &\ge p_{\theta^{(t)}}(\hat{\mathbf z}^{(t+1)}\mid x_i^{(j)}) \\
    &=\ell(\theta^{(t)},\hat{\mathbf z}^{(t+1)}).
\end{align*}
Combining the two inequalities yields
$$
\ell(\theta^{(t+1)},\hat{\mathbf z}^{(t+1)})
\;\ge\;
\ell(\theta^{(t+1)},\hat{\mathbf z}^{(t)})
\;\ge\;
\ell(\theta^{(t)},\hat{\mathbf z}^{(t)}),
$$
which proves the monotonicity.
\end{proof}

Notice that we are using a weighted maximization in \Frameworkname{}++. 
If the maximization uses row-level weights $w_i^{(t)}$ (computed after the Expectation) and maximizes $\sum_{(i,j)\in \mathcal{E}}w_i^{(t)}\log p_\theta(\hat z_{ij}^{(t)}\mid x_i^{(j)})$, the same block-coordinate argument shows monotonic non-decrease of the corresponding weighted objective within iteration $t$ (with $w^{(t)}$ treated as fixed during the maximization), so we omit the similar proof here.

\subsection{Guarantees of Confident Learning}
\label{subsec:cl-theory}

We now analyze the effectiveness of the SLM. We analyze one fixed EM iteration and omit the superscript $t$ for simplicity.
Recall that for each detected erroneous cell $(i,j)\in\mathcal{E}$, we extract the top-$K$ first-token candidates and their probabilities $q_{ij}(r)$, compute a token-dependent threshold $T_j(v)$, and keep a candidate only if its probability exceeds the corresponding threshold. 
The corresponding probability is then used as the cell confidence $c_{ij}$, and row weights $w_i$ are obtained by aggregating $\{c_{ij}\}_{j=1}^d$.
Then, maximization is performed to maximize the row-weighted log-likelihood.

\begin{theorem}[Threshold reduces error rate]
\label{thm:cl_threshold}
Assume (Ranking consistency) that within each predicted first token, the softmax probability $q$ is an order-consistent score: a higher $q$ should not correspond to a higher error probability. This is a weak condition and can be empirically verified.

The threshold $T_j(v)$ reduces the conditional error probability, that is:
$$
P(\hat z_{ij} \neq z_{ij} \mid q_{ij} \ge T_j(v), \hat a_{ij}=v) \le P(\hat z_{ij} \neq z_{ij}\mid \hat a_{ij}=v).
$$
We treat the above probability as a function of $q$ for the following proof.
\end{theorem}

\begin{proof}
Let $A$ be the event "$\hat z_{ij}\neq z_{ij}$", $B,C$ be the event "$q_{ij}\ge T_j(v)$" and "$\hat a_{ij}=v$". Let $f_q(\cdot)$ be the probability mass function of $q_{ij}$.
By the law of total probability, we have
$$
P(A\,|\,C) = P(B)P(A\,|\,B,C) + P(B^c)P(A\,|\,B^c,C).
$$
For simplicity, let $n=P(q_{ij}\ge T_j(v))\in (0,1)$ and define
$$
m_1 = P(A\,|\,B,C), \qquad m_2=P(A\,|\,B^c,C).
$$
Then,
$$
P(A\,|\,C) =n m_1+(1-n)m_2,
$$
and we have
$$
P(A\,|\,C) - P(A\,|\,B,C) = (1-n)(m_2-m_1).
$$
Using the ranking consistency, $P(\hat z_{ij} \neq z_{ij}\mid q_{ij}=q, \hat a_{ij}=v)$ is non-increasing in $q$. We denote it by $g(q)$, then $m_1$ and $m_2$ are the conditional expectation:
\begin{align*}
    m_1 &= \frac{\int^1_{T_j(v)}P(A\,|\,q_{ij}=q, C)f_q(q)\mathrm{d}q}{\int^1_{T_j(v)}f_q(q)\mathrm{d}q}=\mathbb{E}(g(q)\,|\,q\ge T_j(v), C)\\
    &\le g(T)\le \mathbb{E}(g(q)\,|\,q\le T_j(v), C)=m_2.
\end{align*}
Thus $m_2-m_1\ge 0$, and we have proved $P(A\,|\,C) \ge P(A\,|\,B,C)$, which is 
$$
% P(\hat z_{ij} \ne z_{ij} \mid q_{ij} \ge T_j(v), \hat a_{ij}=v) \le P(\hat z_{ij} \ne z_{ij}\mid \hat a_{ij}=v)，
P(\hat z_{ij}\ne z_{ij} \mid q_{ij} \ge T_j(v),\hat a_{ij}=v) \leq P(\hat z_{ij}\ne z_{ij} \mid \hat{a}_{ij}=v),
$$
Exactly the desired inequality.
\end{proof}

We also demonstrate that the weighted data yields a gradient closer to the true gradient for parameter updates compared to the original data.

\begin{theorem}[Restatement of weighted update effectiveness]
\label{thm:cl_grad_full}
For each row $i$, define the log-likelihood loss
$$
\hat \ell_i(\theta) = \sum_{(i,j)\in\mathcal{E}}-\log p_\theta(\hat z_{ij}\mid x_i^{(j)}),
$$
and the corresponding (unknown clean label) loss
$$
\ell^\ast_i(\theta) = \sum_{(i,j)\in\mathcal{E}}-\log p_\theta( z_{ij}\mid x_i^{(j)}).
$$
Let $\hat g_i(\theta)=\nabla_\theta \hat \ell_i(\theta)$ and $g_i^\ast(\theta)=\nabla_\theta \ell_i^\star(\theta)$.
Assume there is a heteroscedastic noise decomposition
$$
\hat g_i(\theta) = g_i^\ast (\theta) + \epsilon_i,
$$
where $\epsilon_i\sim N(\mu_i, \sigma^2/\omega_i)$, and $\{\epsilon_i\}_{i=1}^n$ are conditionally independent. Without loss of generality, we can assume $\mu_i=0$.
Recall that $\omega_i^{\ast}$ is the normalized row-level weight.
Define the weighted gradient $\hat g_{\omega}$, unweighted (uniform weighted) gradient $\hat g_{u}$ and the true gradient $g^\ast$ as 
$$
\hat g_{\omega}(\theta)=\sum_{i=1}^n \omega_i^\ast \hat g_i(\theta),
\quad
\hat g_{u}(\theta)=\frac1n\sum_{i=1}^n \hat g_i(\theta),
\quad
g^\ast(\theta)=\frac1n\sum_{i=1}^n g_i^\ast(\theta).
$$
Then, for any fixed $\theta$,
$$
\mathbb{E}\|\hat g_{\omega}(\theta)-g^\ast(\theta)\| \leq \mathbb{E}\|\hat g_u(\theta)-g^\ast(\theta)\|.
$$
\end{theorem}

\begin{proof}
With $\theta$ fixed, we have
$$
\mathbb{E}\|\hat g_u(\theta)-g^\ast(\theta)\|=\frac{1}{n^2}\sum_{i=1}^n \mathbb{E}\|\epsilon_i\|= \frac{\sigma^2}{n^2}\sum_{i=1}^n\frac{1}{\omega^\ast_i}.
$$
Similarly,
$$
\mathbb{E}\|\hat g_\omega(\theta)-g^\ast(\theta)\|=\sum_{i=1}^n \mathbb{E}(\omega_i^{\ast2}\epsilon_i^2)= \sigma^2.
$$
By the Cauchy-Schwarz inequality,
$$
\left(\sum_{i=1}^n \omega^\ast_i\right)\left(\sum_{i=1}^n \frac1{\omega_i^\ast}\right)\ge n^2
\quad\Longrightarrow\quad
1\le \frac1{n^2}\sum_{i=1}^n \frac1{\omega^\ast_i}.
$$
Finally we proved
$$
\mathbb{E}\|\hat g_{\omega}(\theta)-g^\ast(\theta)\| \leq \mathbb{E}\|\hat g_u(\theta)-g^\ast(\theta)\|.
$$
The equality case happens when $\omega_1=\dots=\omega_n$.
\end{proof}
